# Supplementary material for: Leveraging Intra-modal and Inter-modal Interaction for Multi-Modal Entity Alignment
Source: arXiv:2404.17590 source file (2024-04-19)
Supplement: Supplementary file 1 [file appendix.tex]

\begin{figure*}[htbp]
  \centering
  % \subcaptionbox{Different of embedding dimension}
  % {\includegraphics[width=0.16\linewidth]{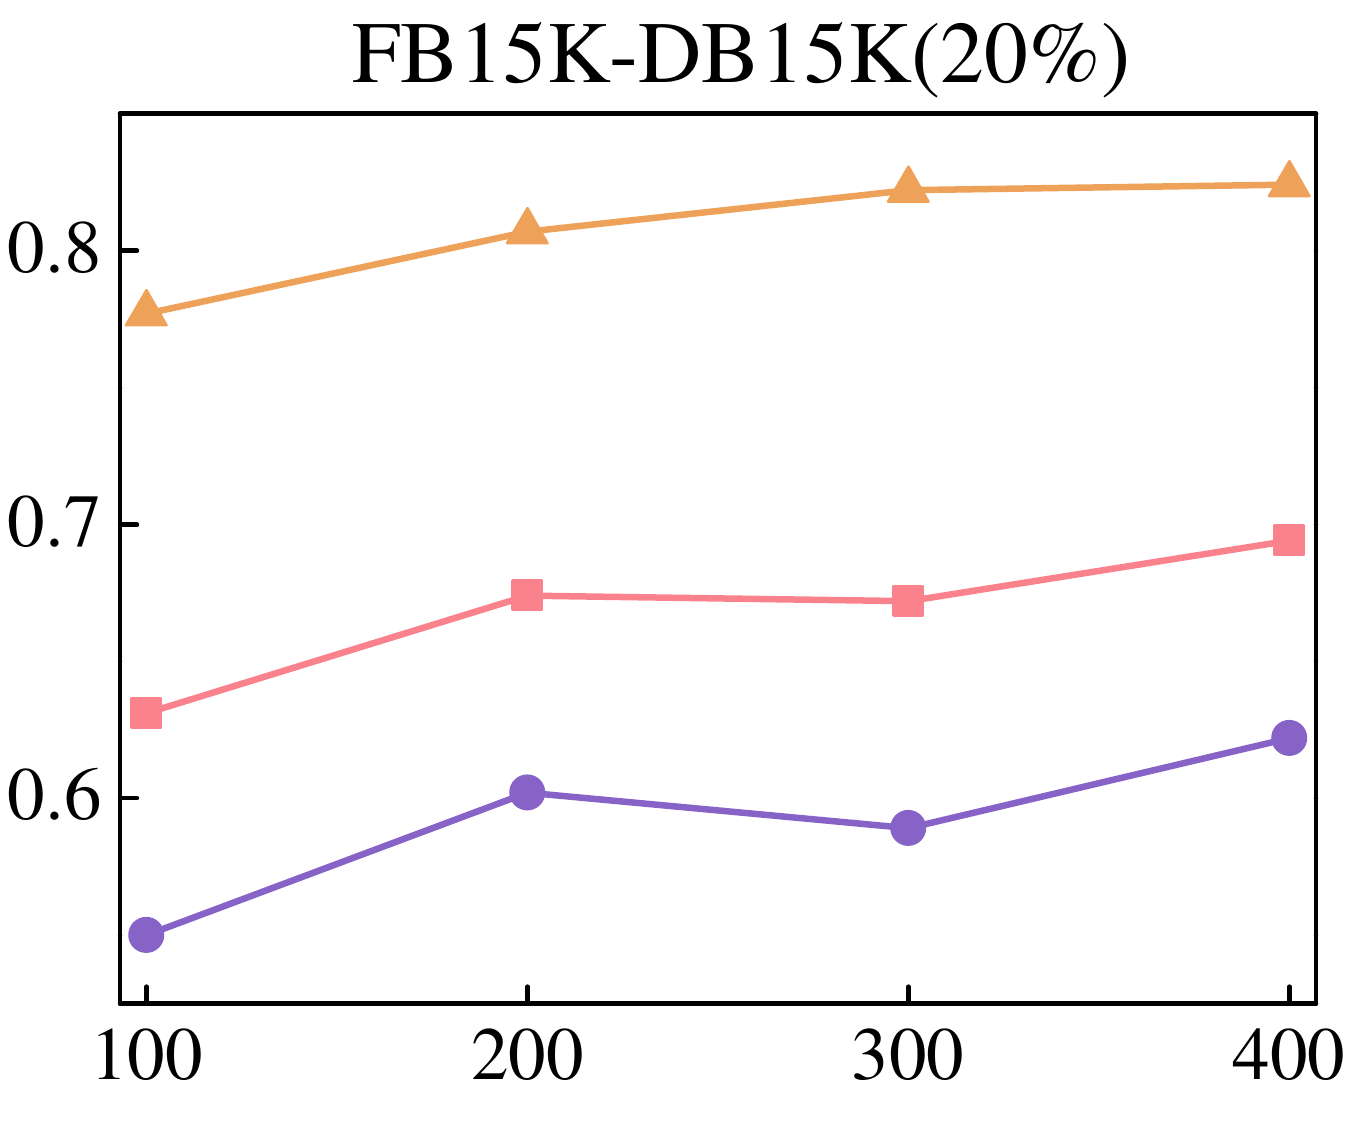}\hfill
  % \includegraphics[width=0.165\linewidth]{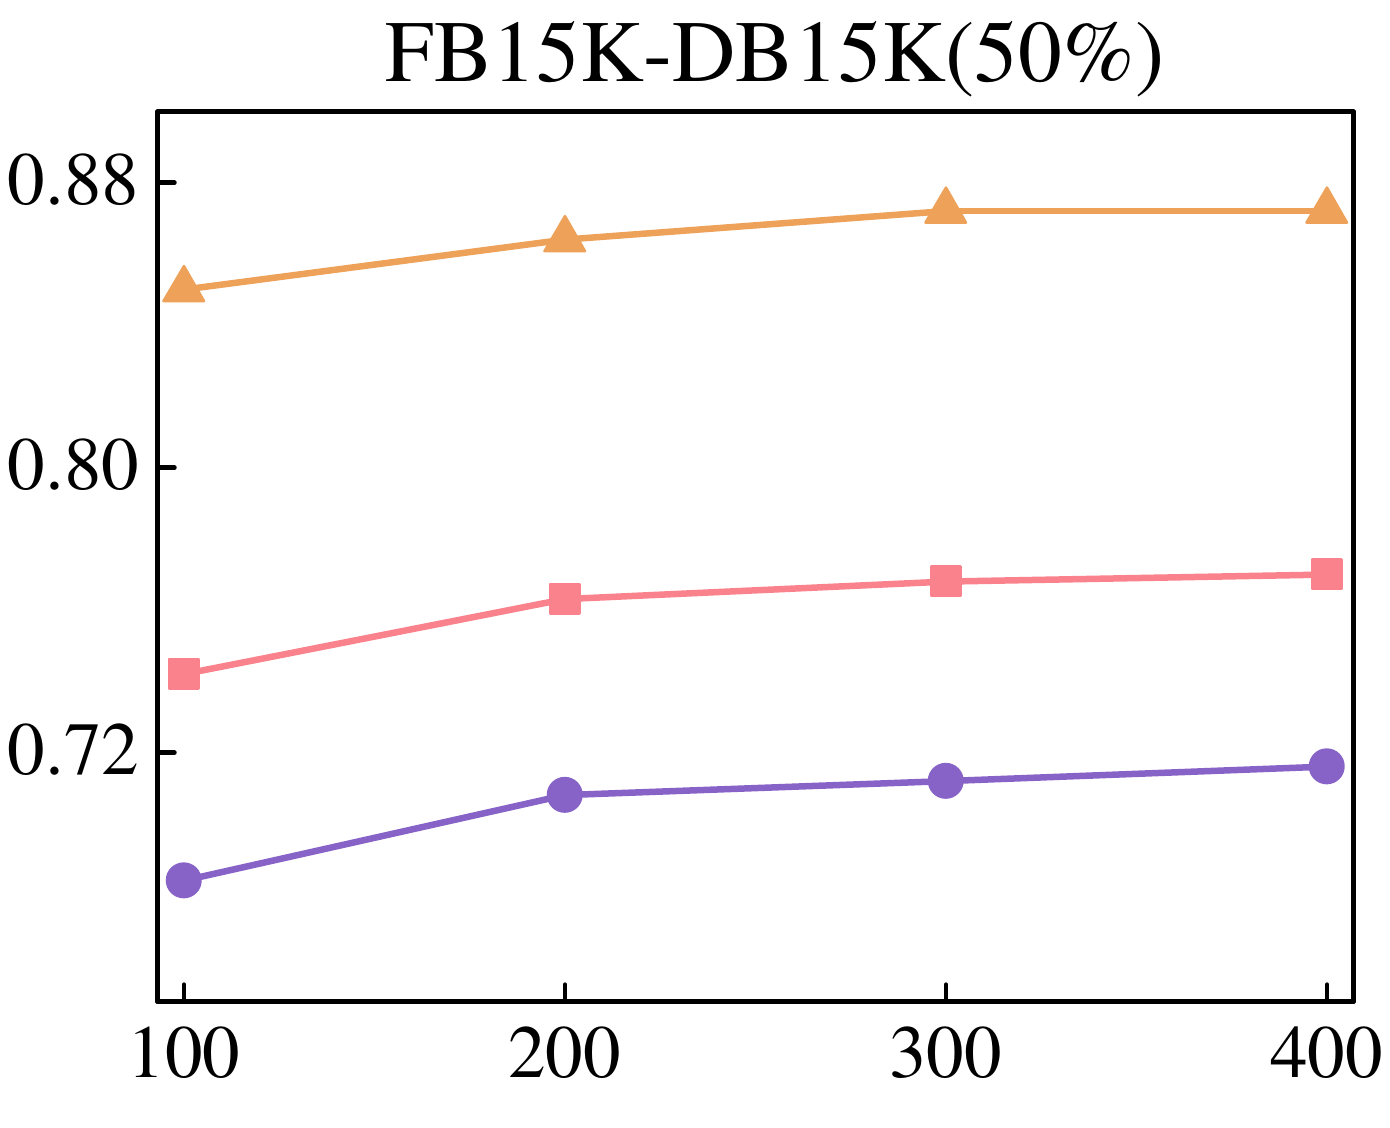}\hfill
  % \includegraphics[width=0.165\linewidth]{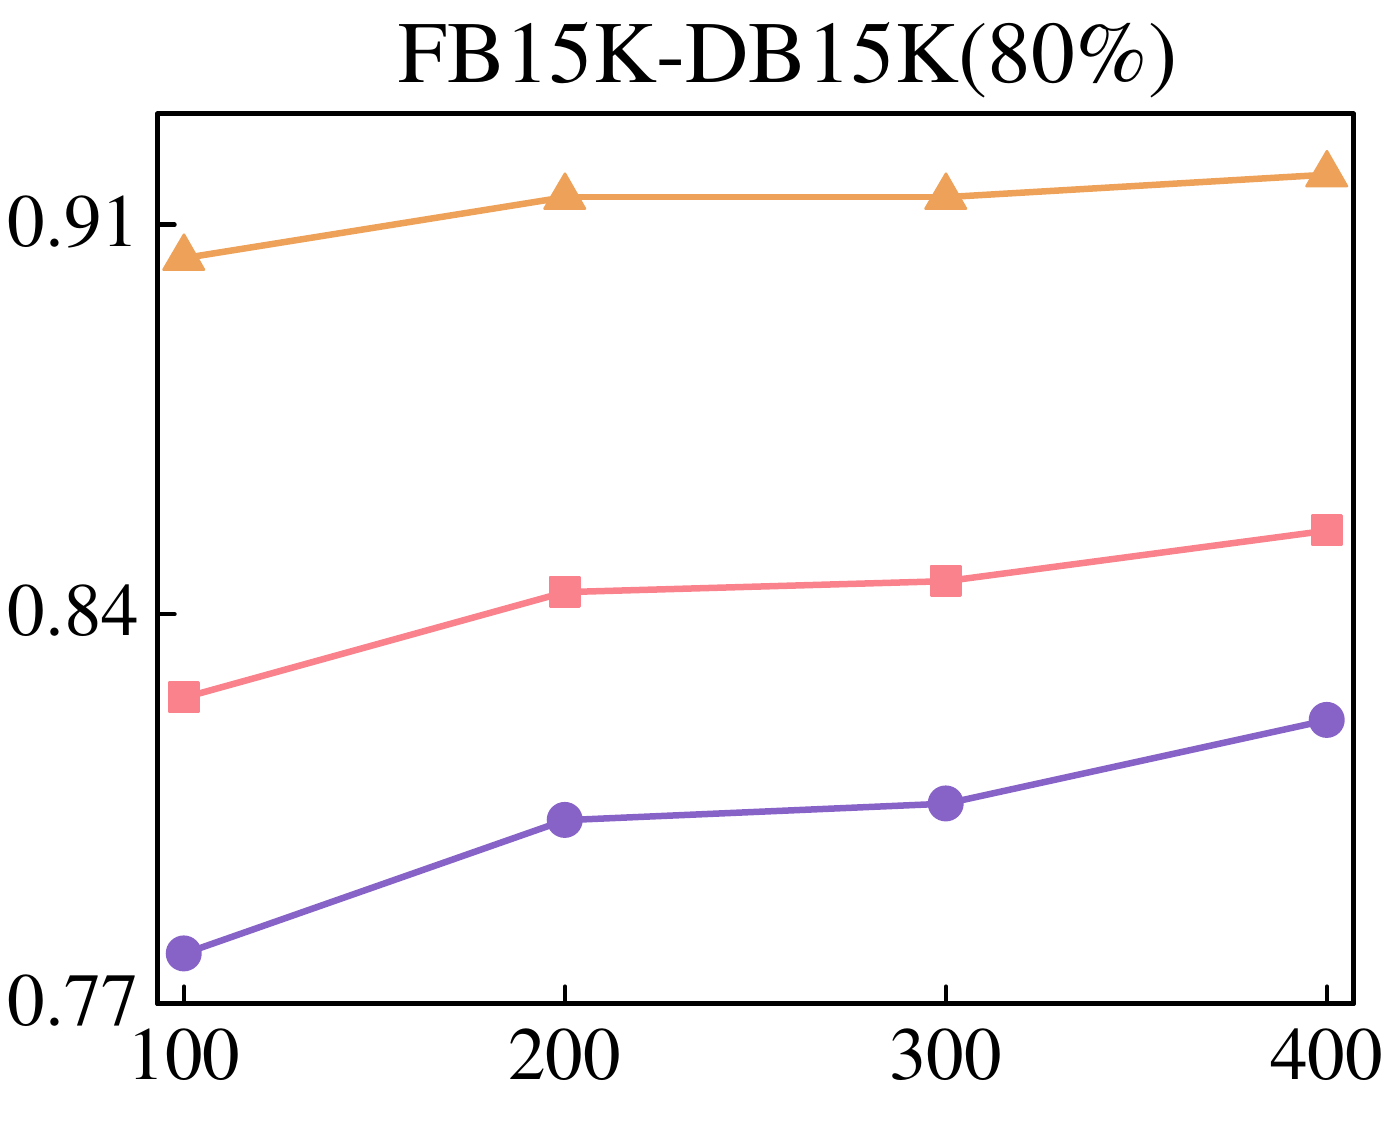}\hfill
  % \includegraphics[width=0.165\linewidth]{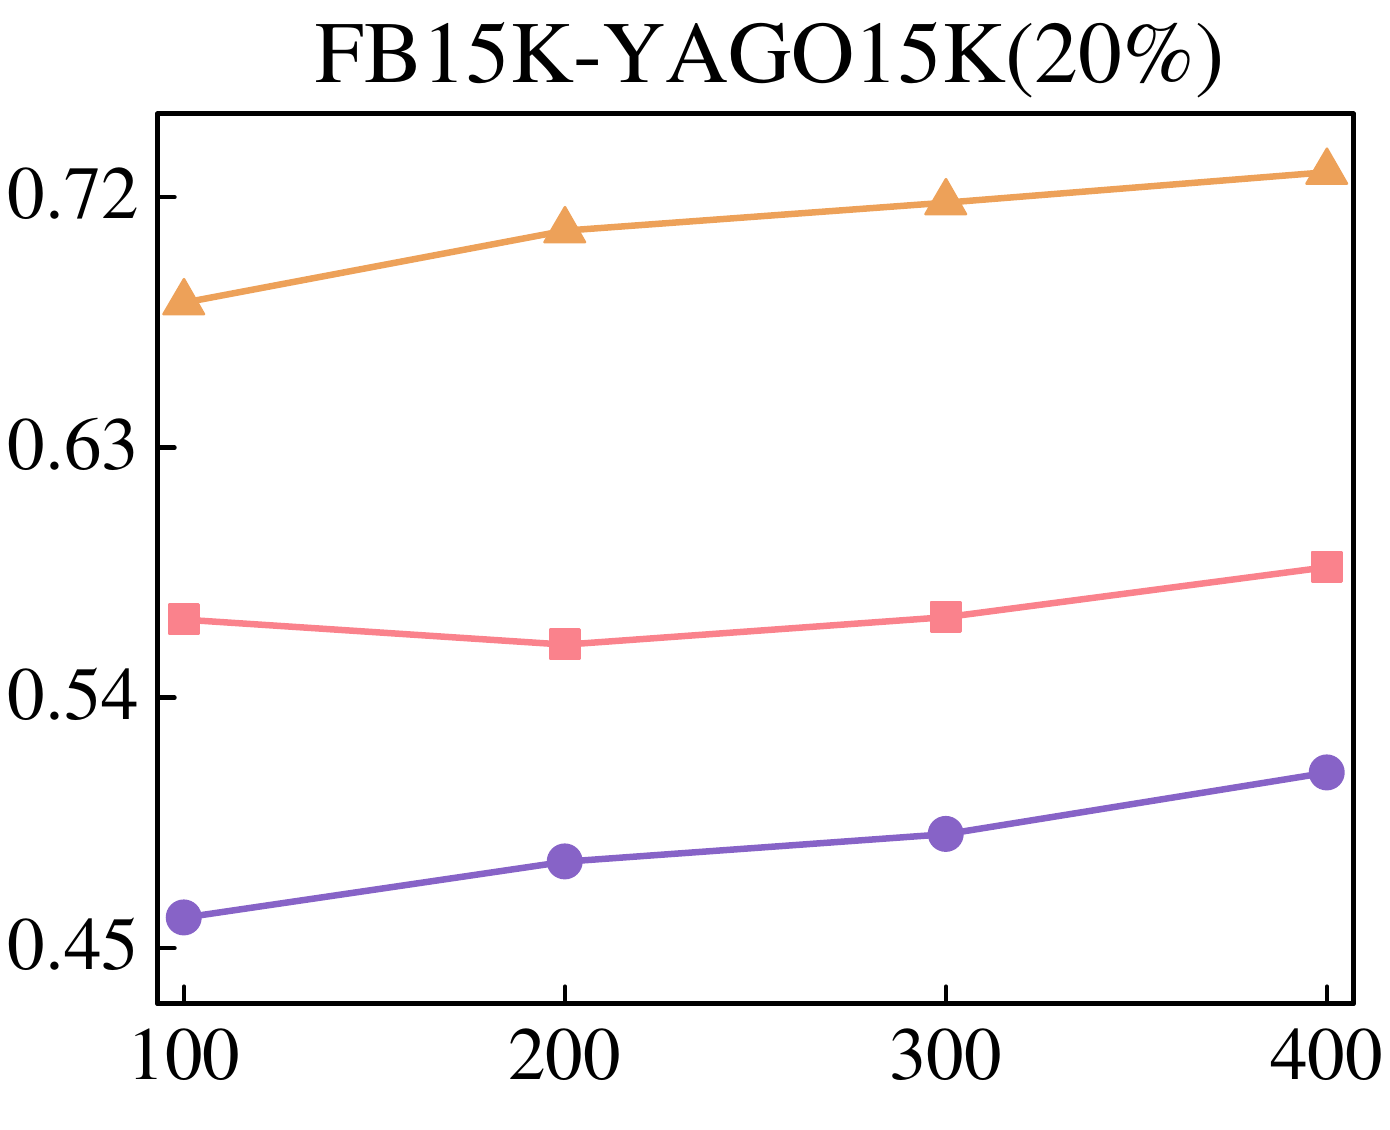}\hfill
  % \includegraphics[width=0.165\linewidth]{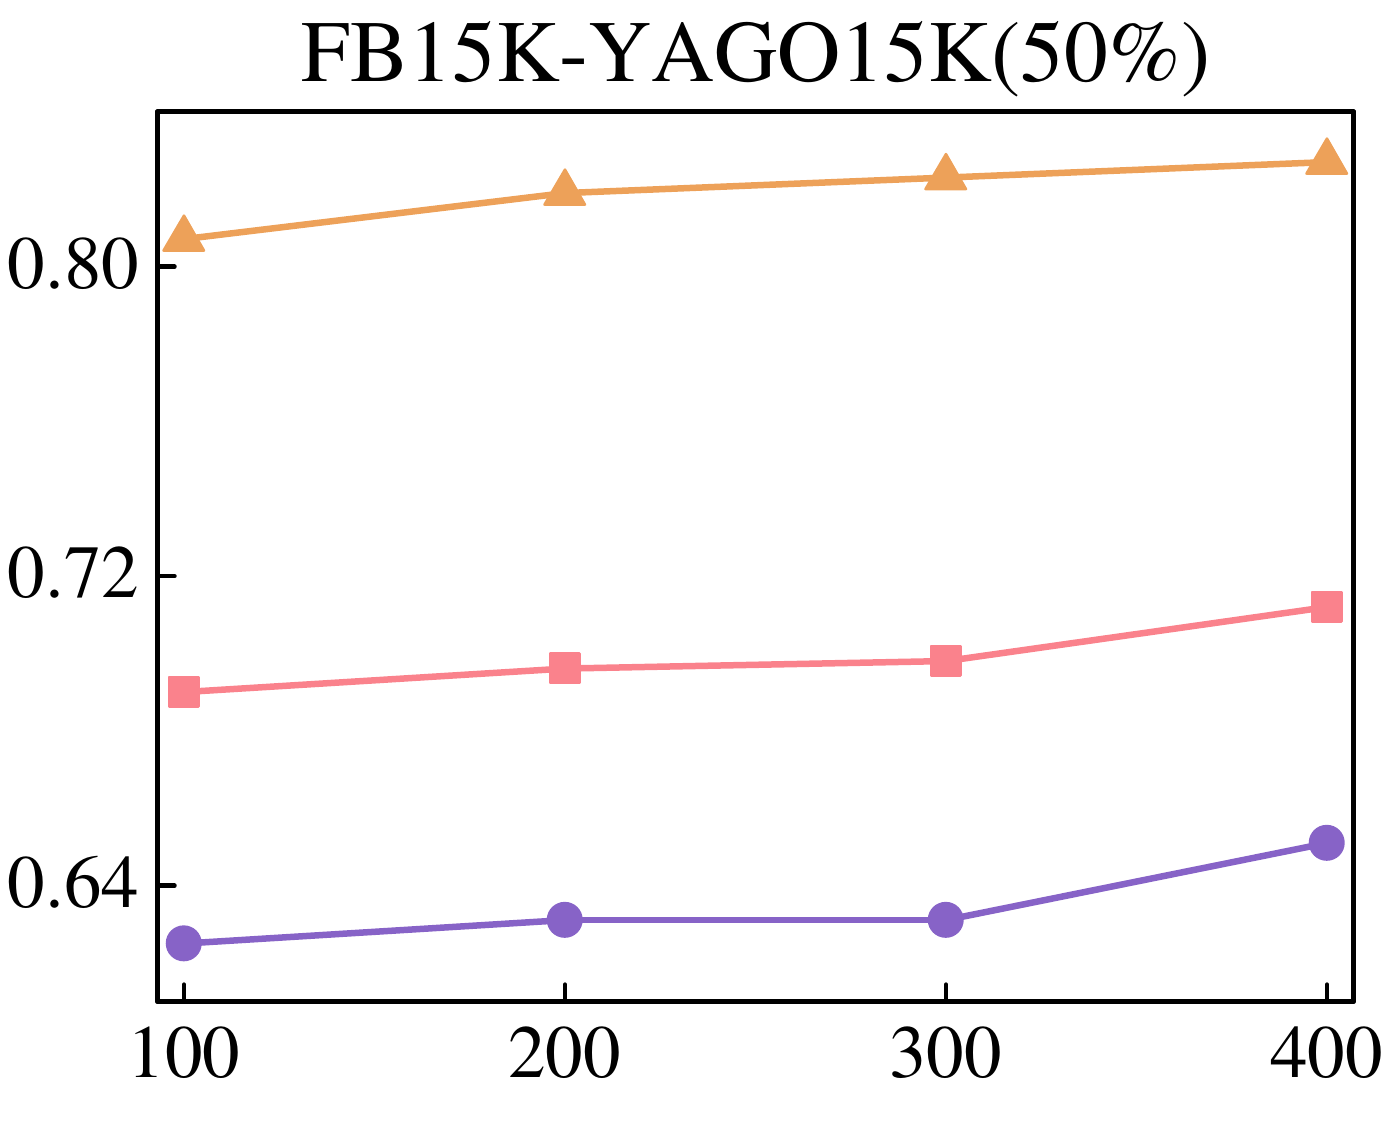}\hfill
  % \includegraphics[width=0.165\linewidth]{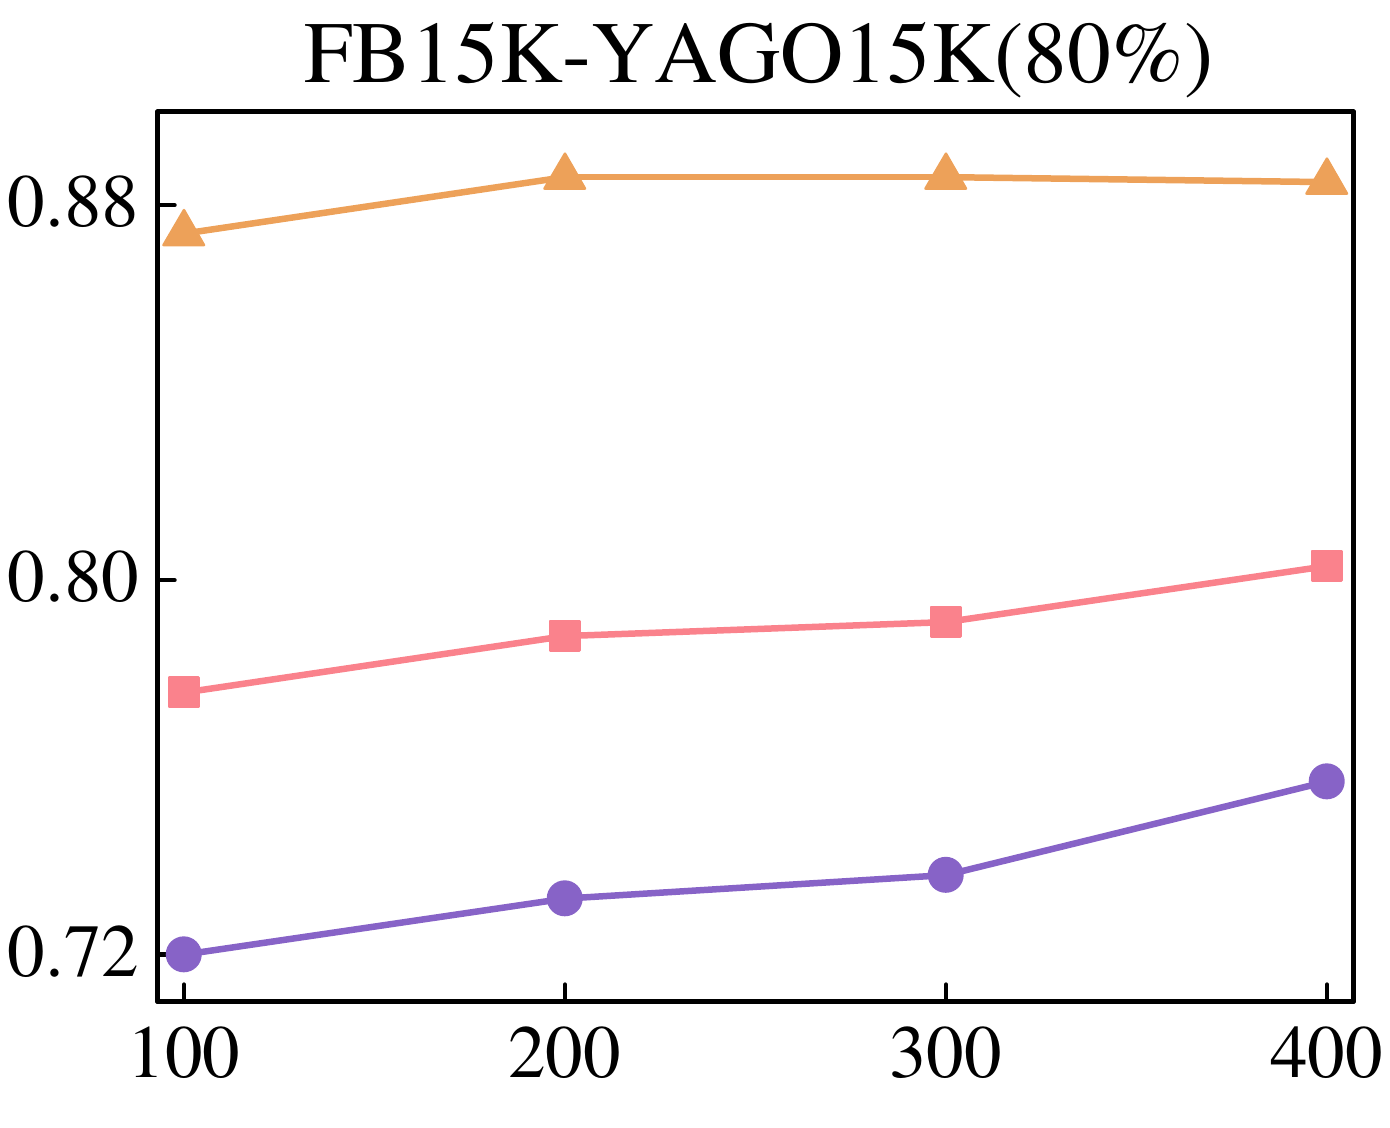}}
  
  % \subcaptionbox{Different of KL weight}
  % {\includegraphics[width=0.16\linewidth]{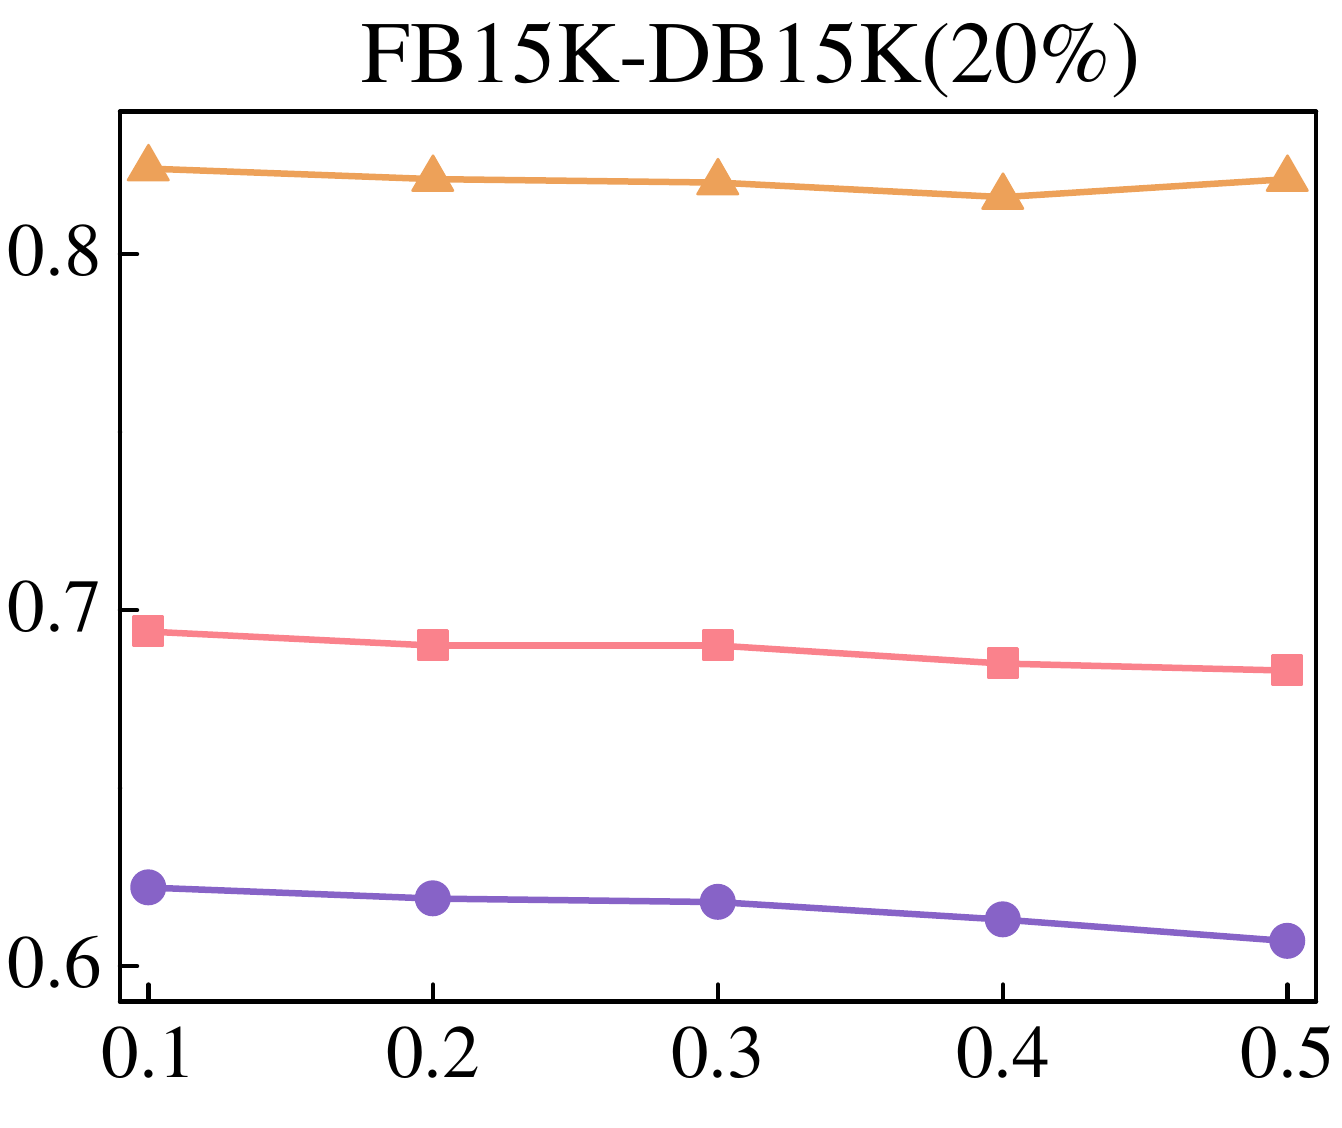}\hfill
  % \includegraphics[width=0.165\linewidth]{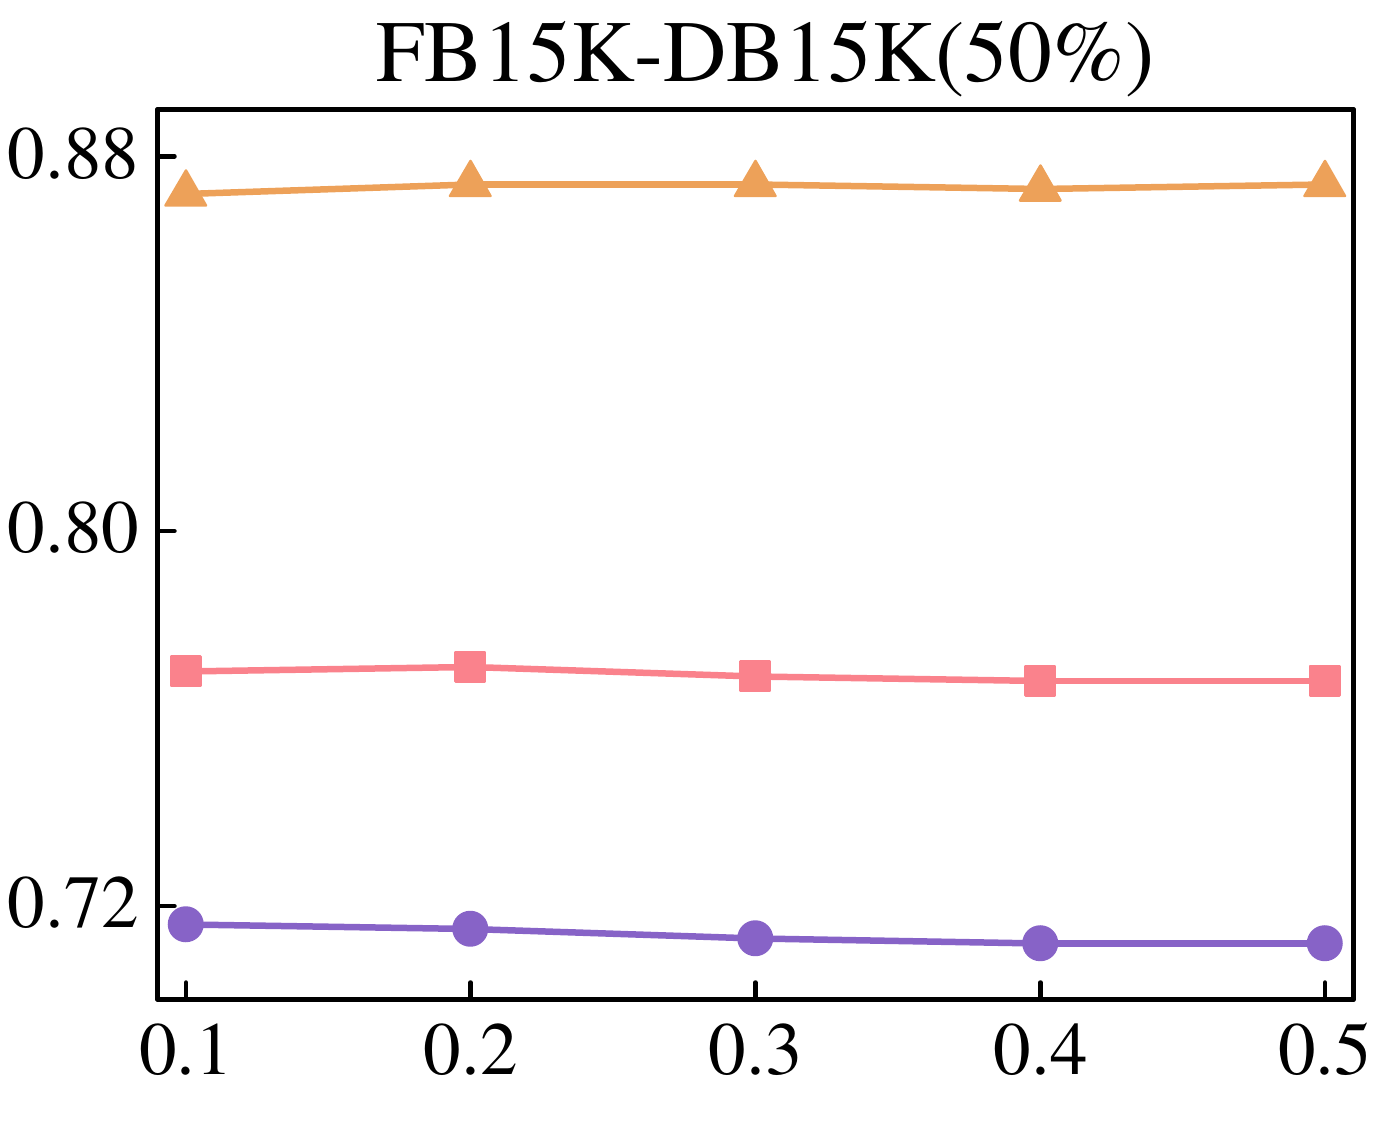}\hfill
  % \includegraphics[width=0.165\linewidth]{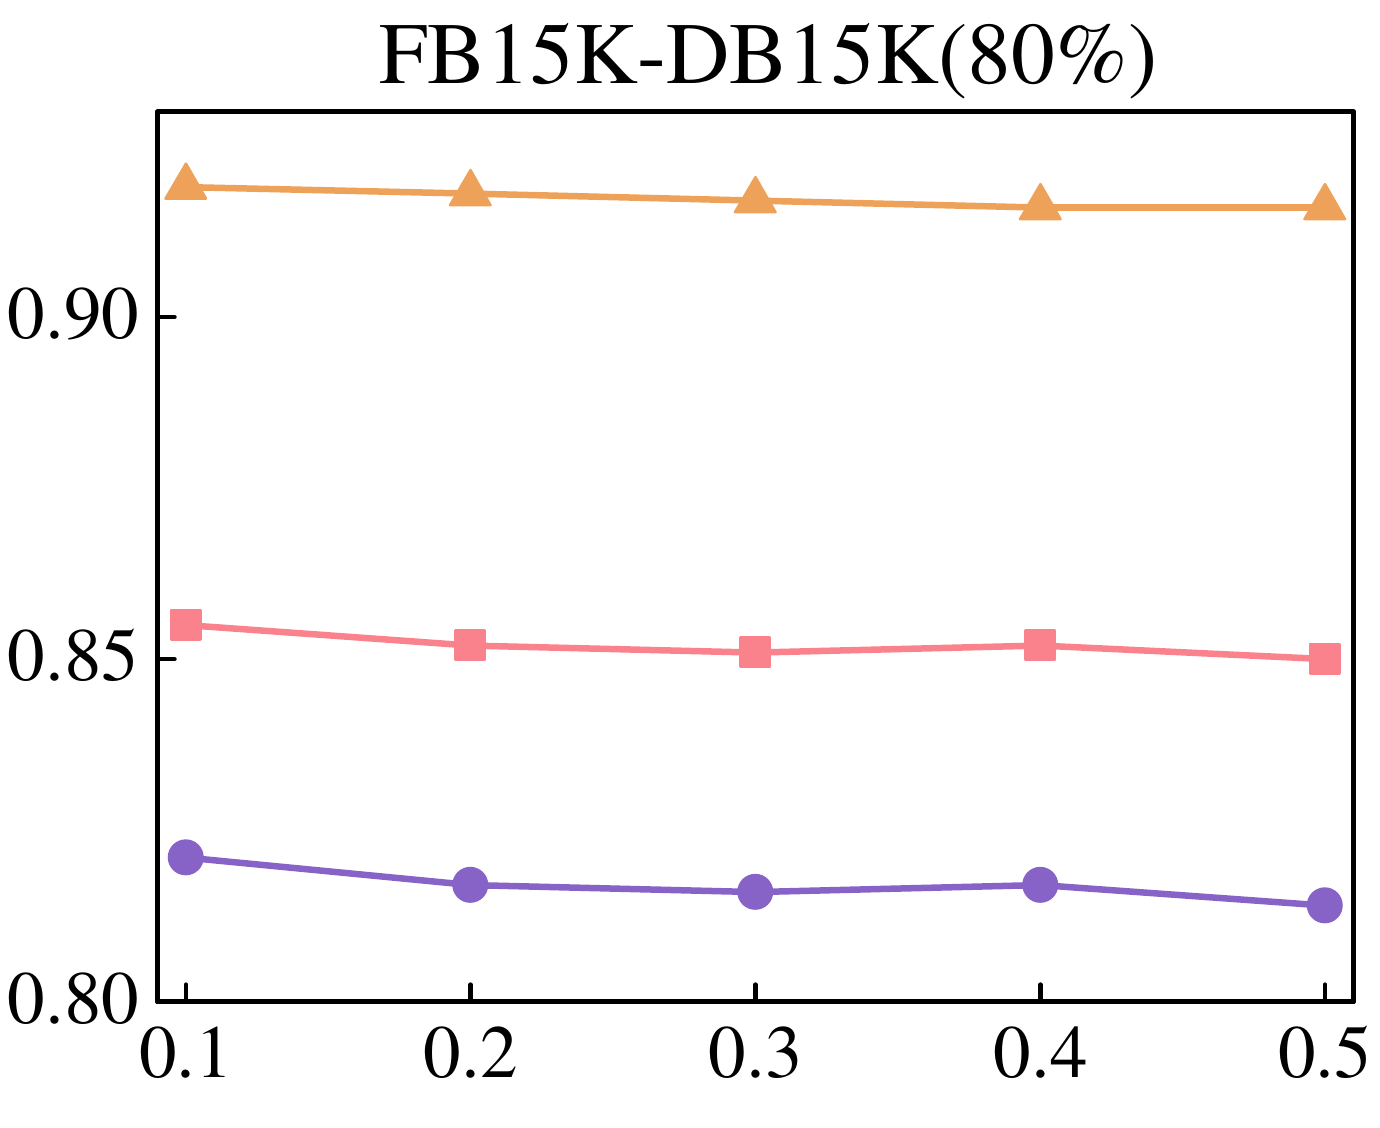}\hfill
  % \includegraphics[width=0.16\linewidth]{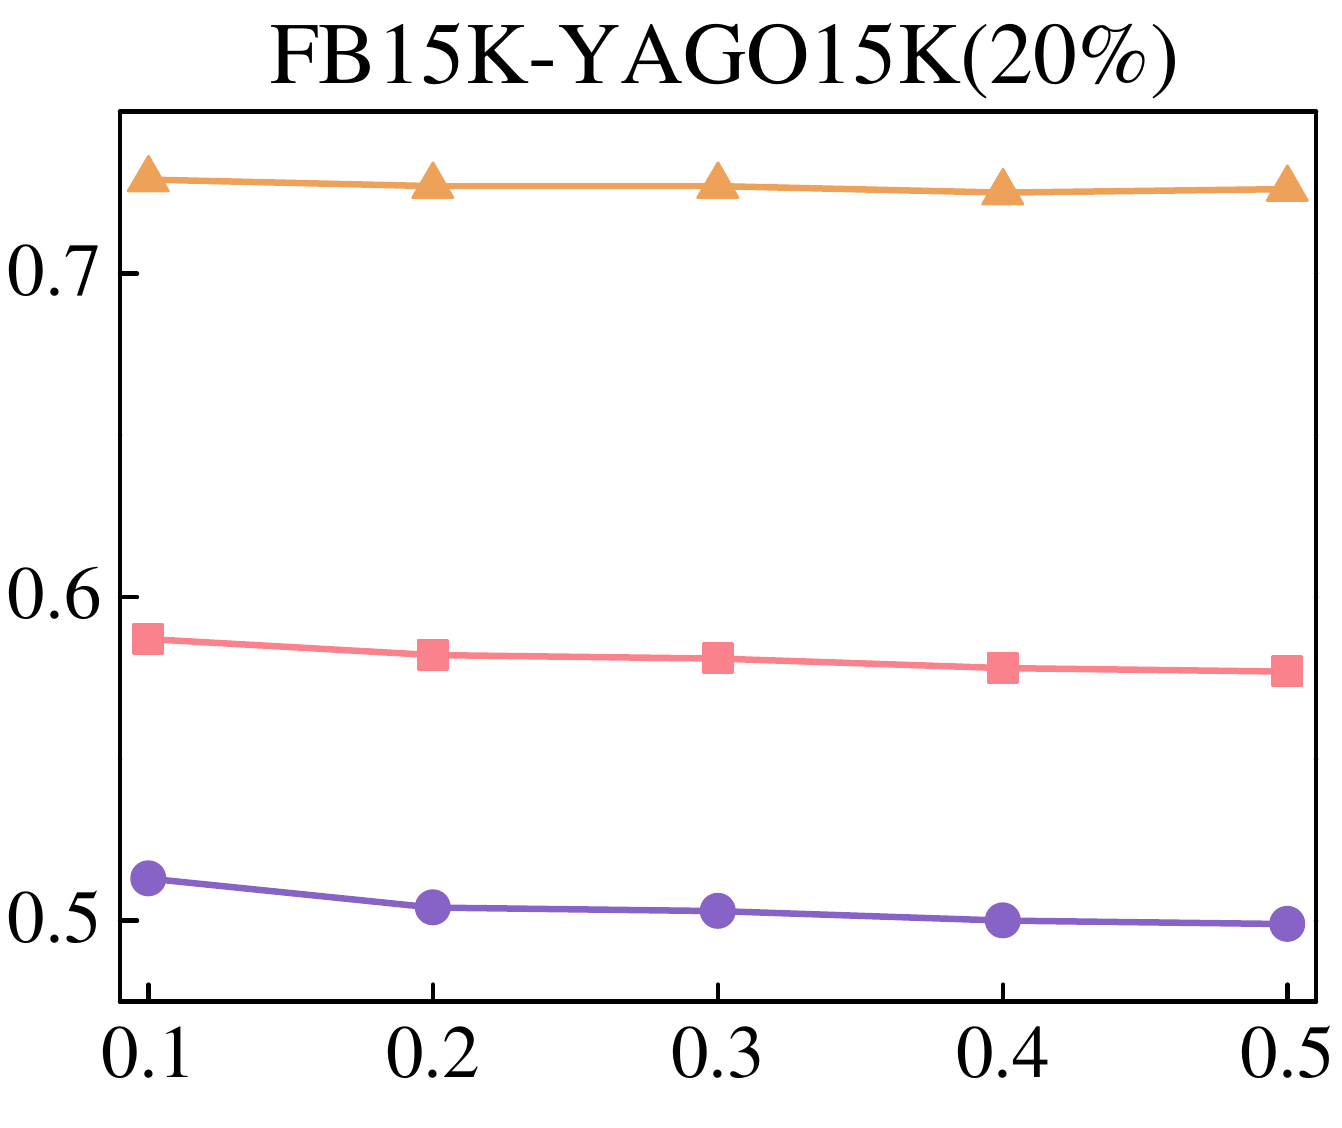}\hfill
  % \includegraphics[width=0.165\linewidth]{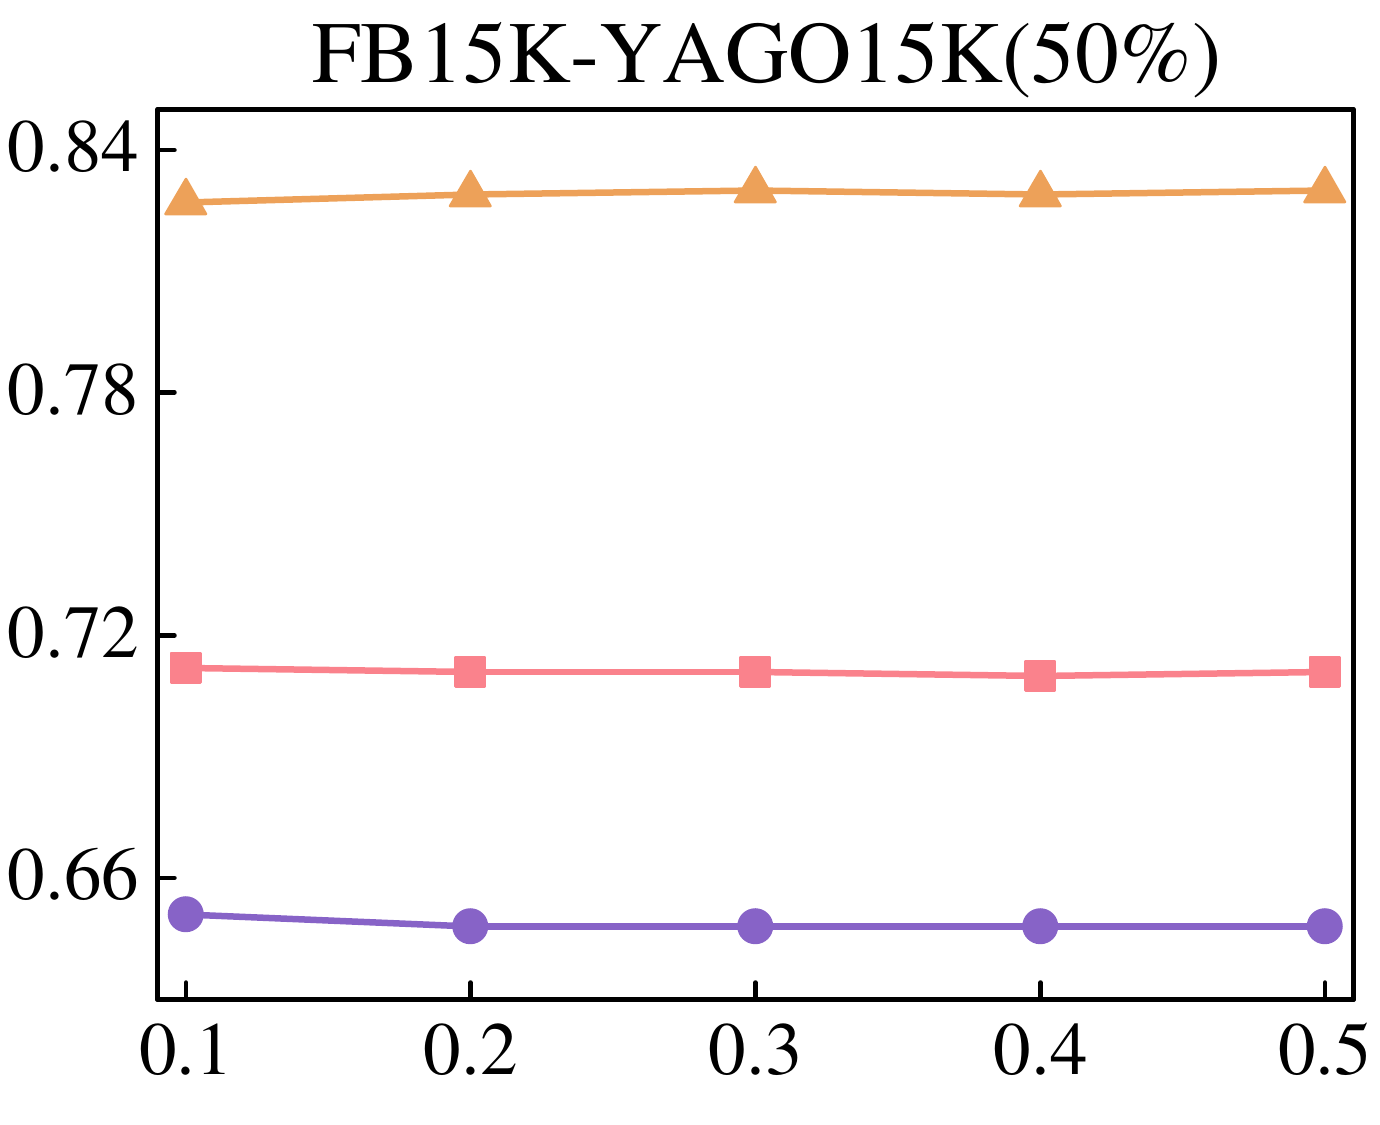}\hfill
  % \includegraphics[width=0.165\linewidth]{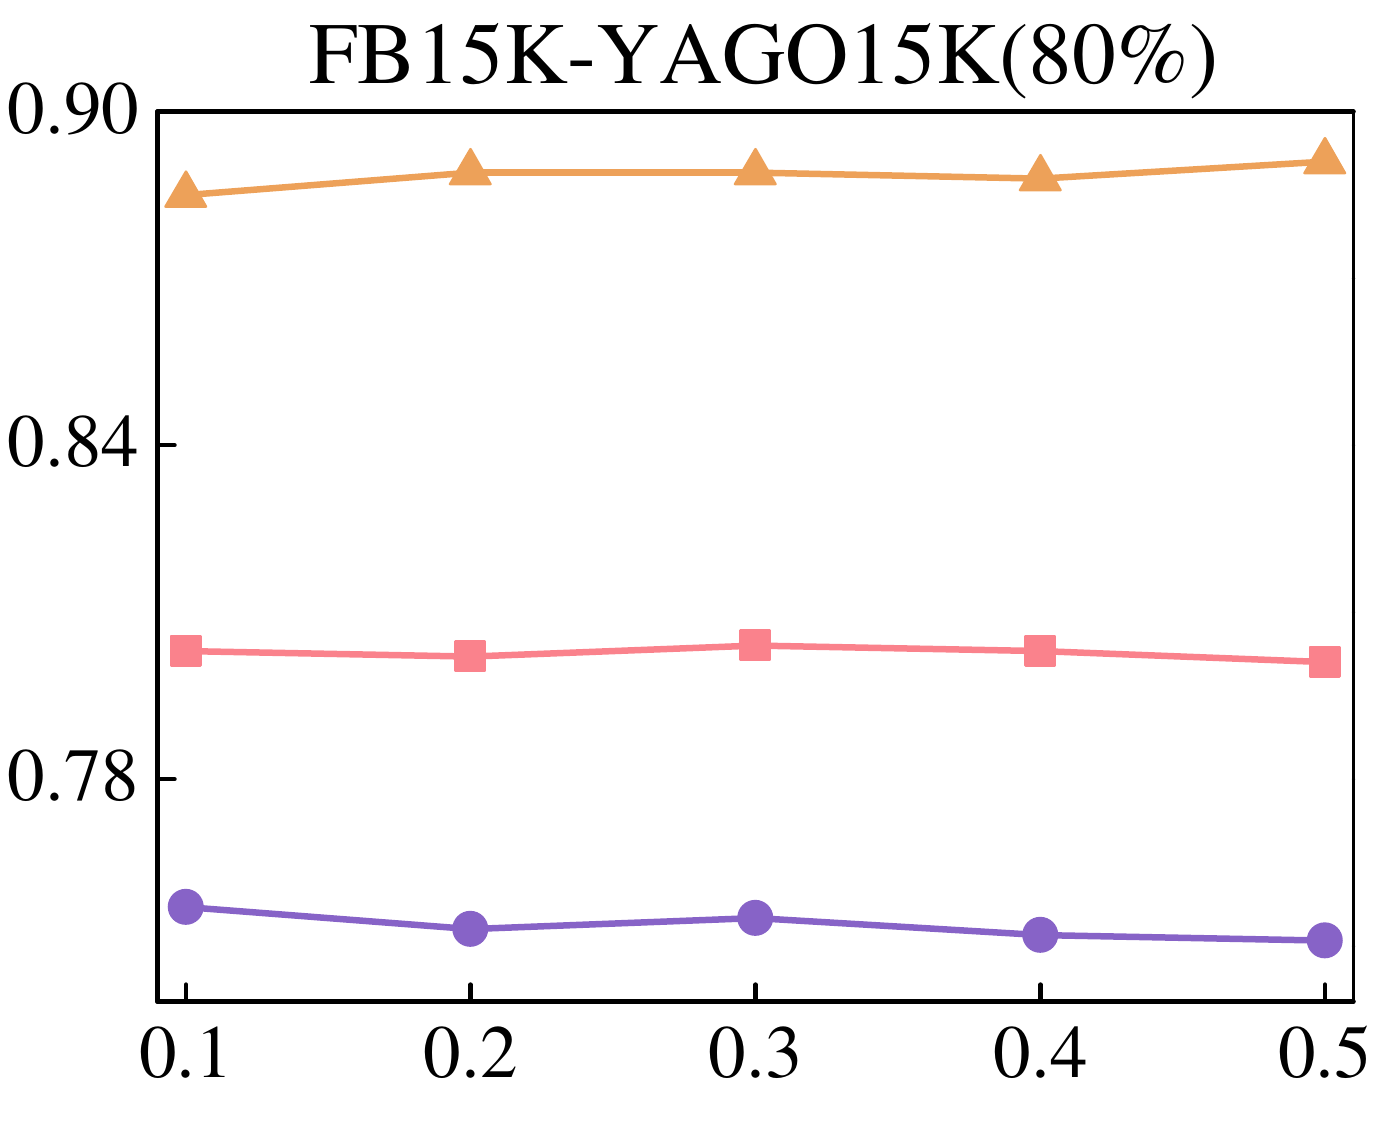}}

  \subcaptionbox{Different Embedding Dimensions $d$}
  {\includegraphics[width=0.16\linewidth]{img/dim_FB15K_DB15K_20.pdf}\hfill
  \includegraphics[width=0.165\linewidth]{img/dim_FB15K_DB15K_50.pdf}\hfill
  \includegraphics[width=0.165\linewidth]{img/dim_FB15K_DB15K_80.pdf}}
  \subcaptionbox{Different Incremental Rates $\lambda$}{
  \includegraphics[width=0.16\linewidth]{img/kl_FB15K_YAGO15K_20.pdf}\hfill
  \includegraphics[width=0.165\linewidth]{img/kl_FB15K_YAGO15K_50.pdf}\hfill
  \includegraphics[width=0.165\linewidth]{img/kl_FB15K_YAGO15K_80.pdf}}

  \subcaptionbox{Different Weight Values $\gamma$}
  {\includegraphics[width=0.165\linewidth]{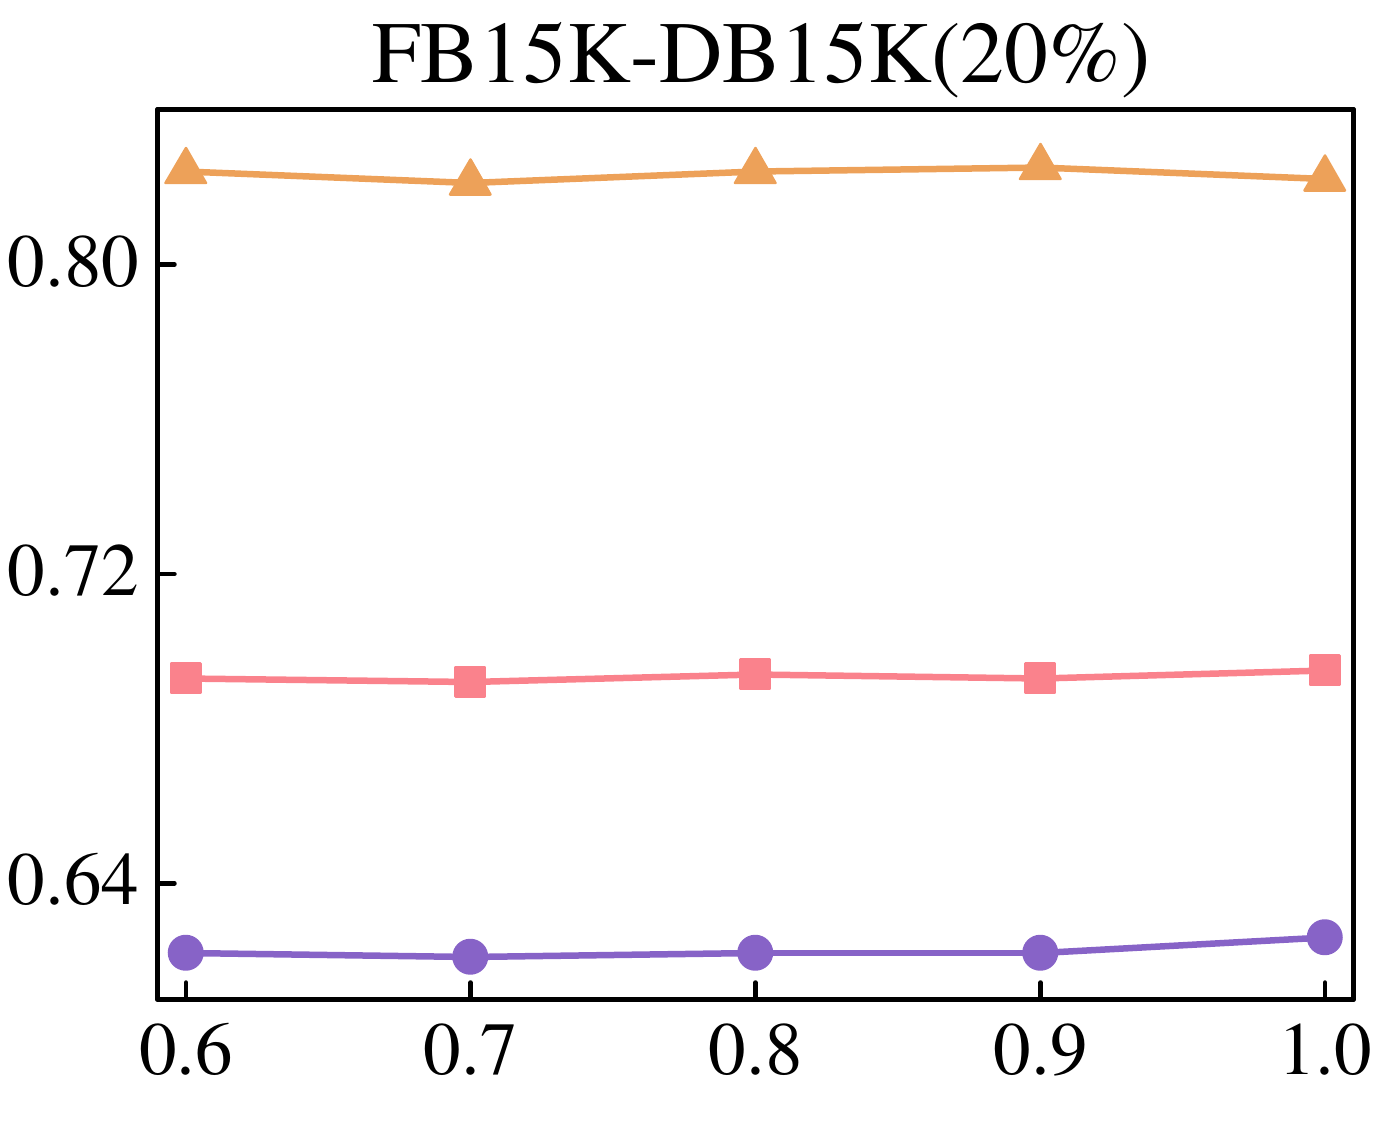}\hfill
  \includegraphics[width=0.165\linewidth]{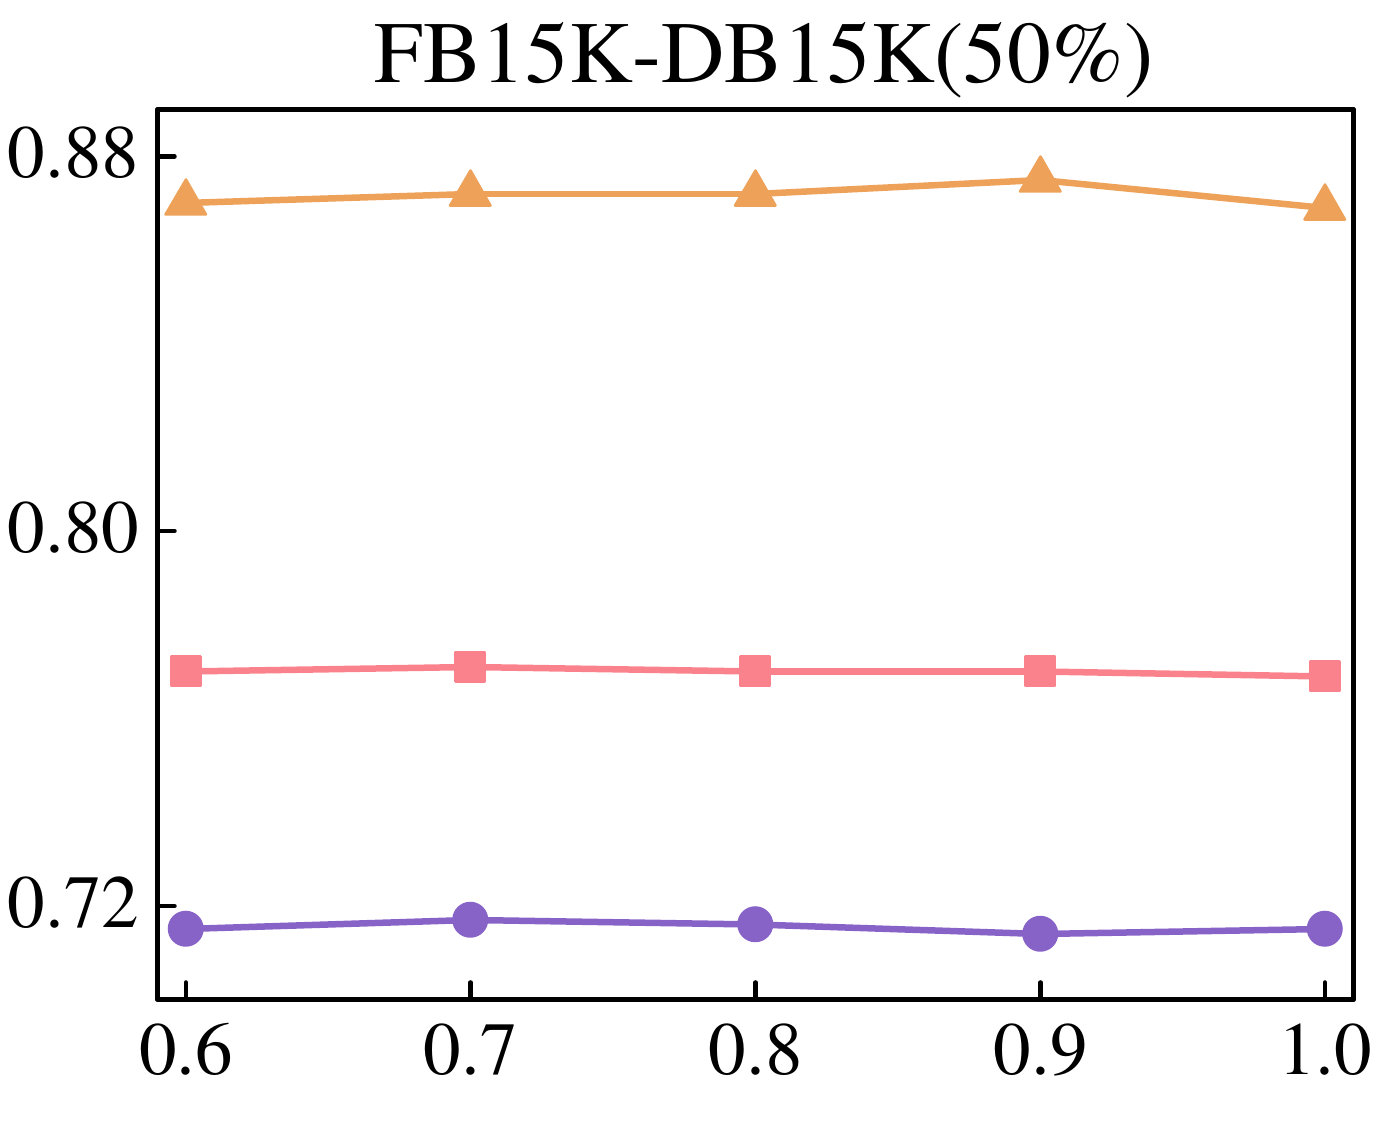}\hfill
  \includegraphics[width=0.165\linewidth]{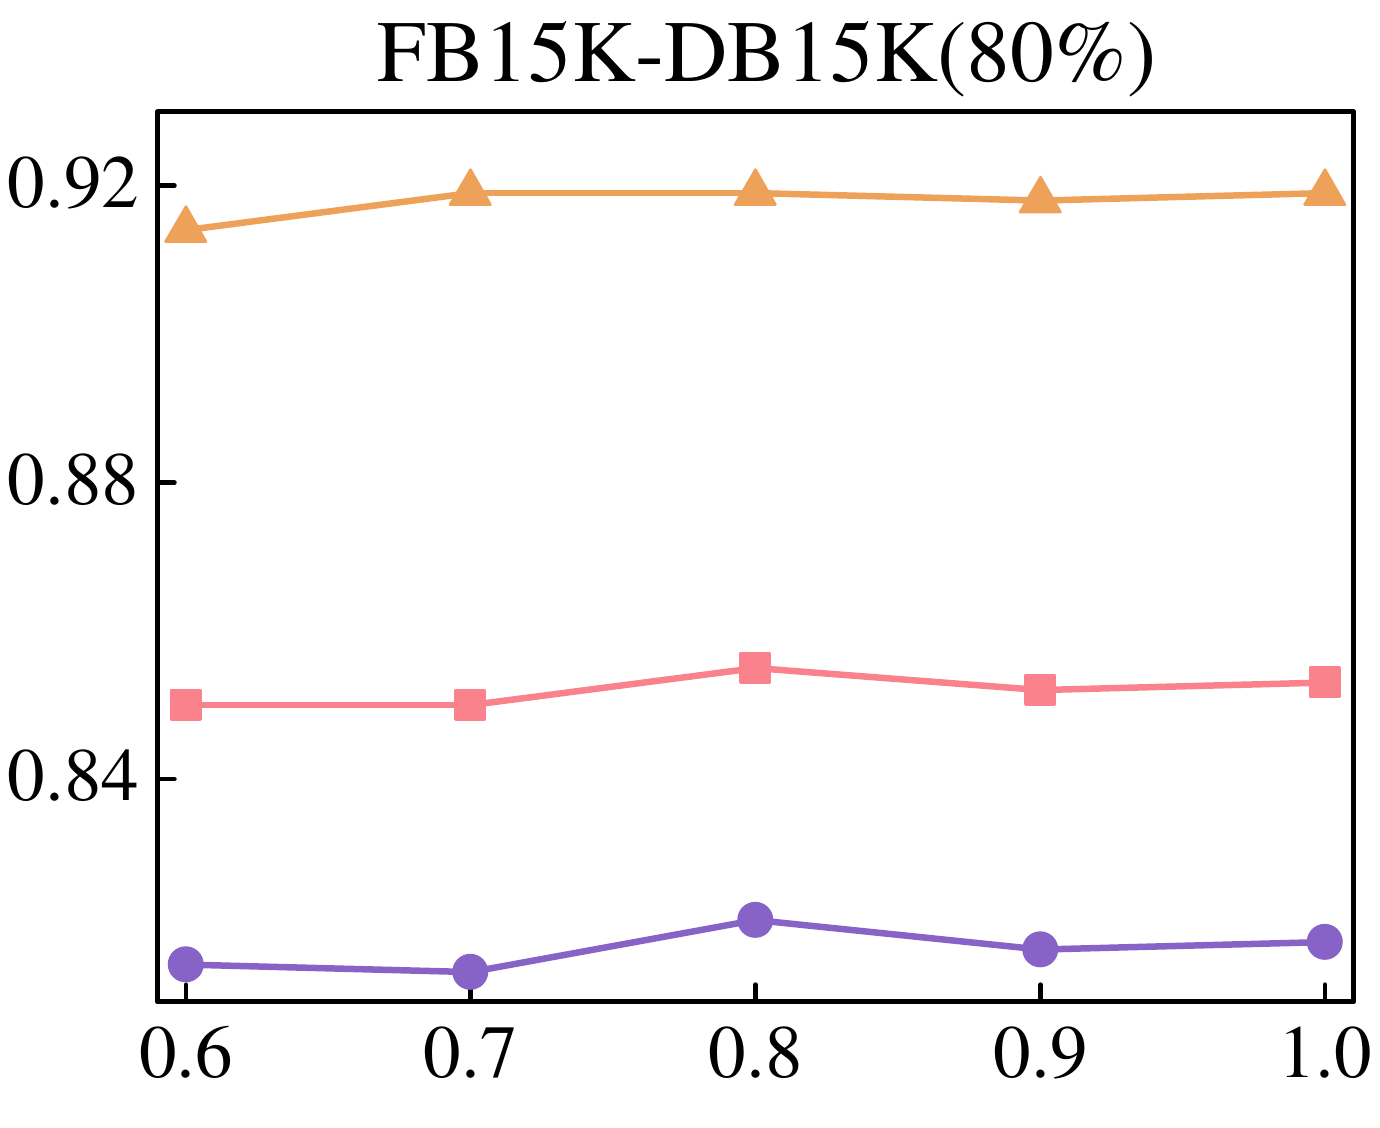}}
  \subcaptionbox{Different Temperature Values $\tau$}{
  \includegraphics[width=0.16\linewidth]{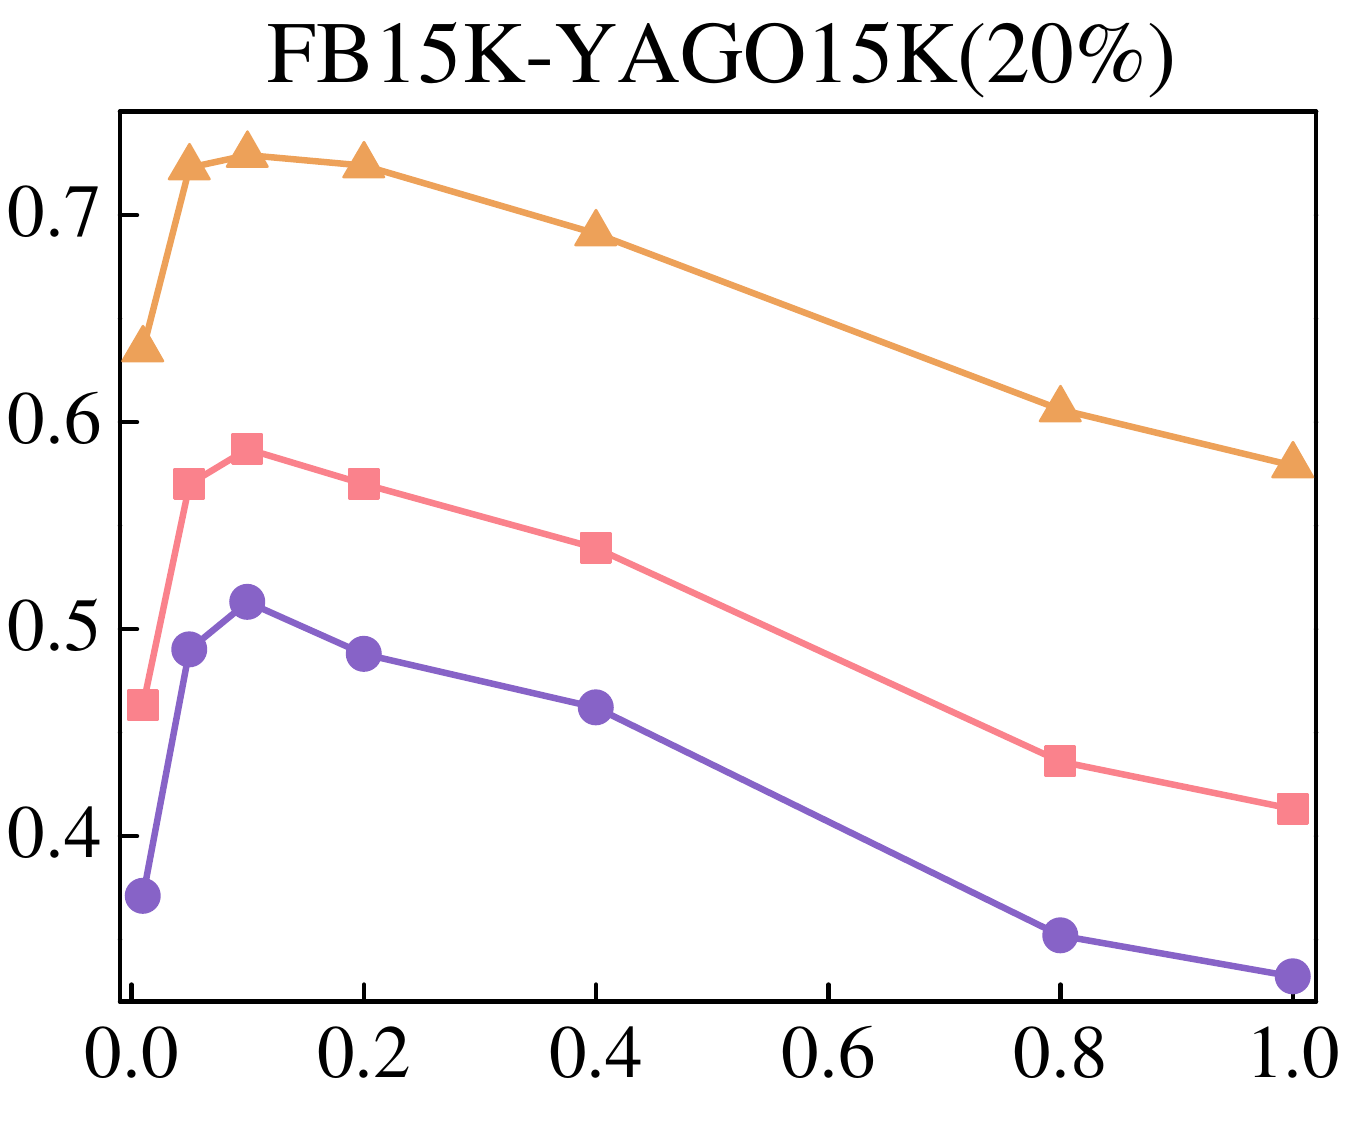}\hfill
  \includegraphics[width=0.16\linewidth]{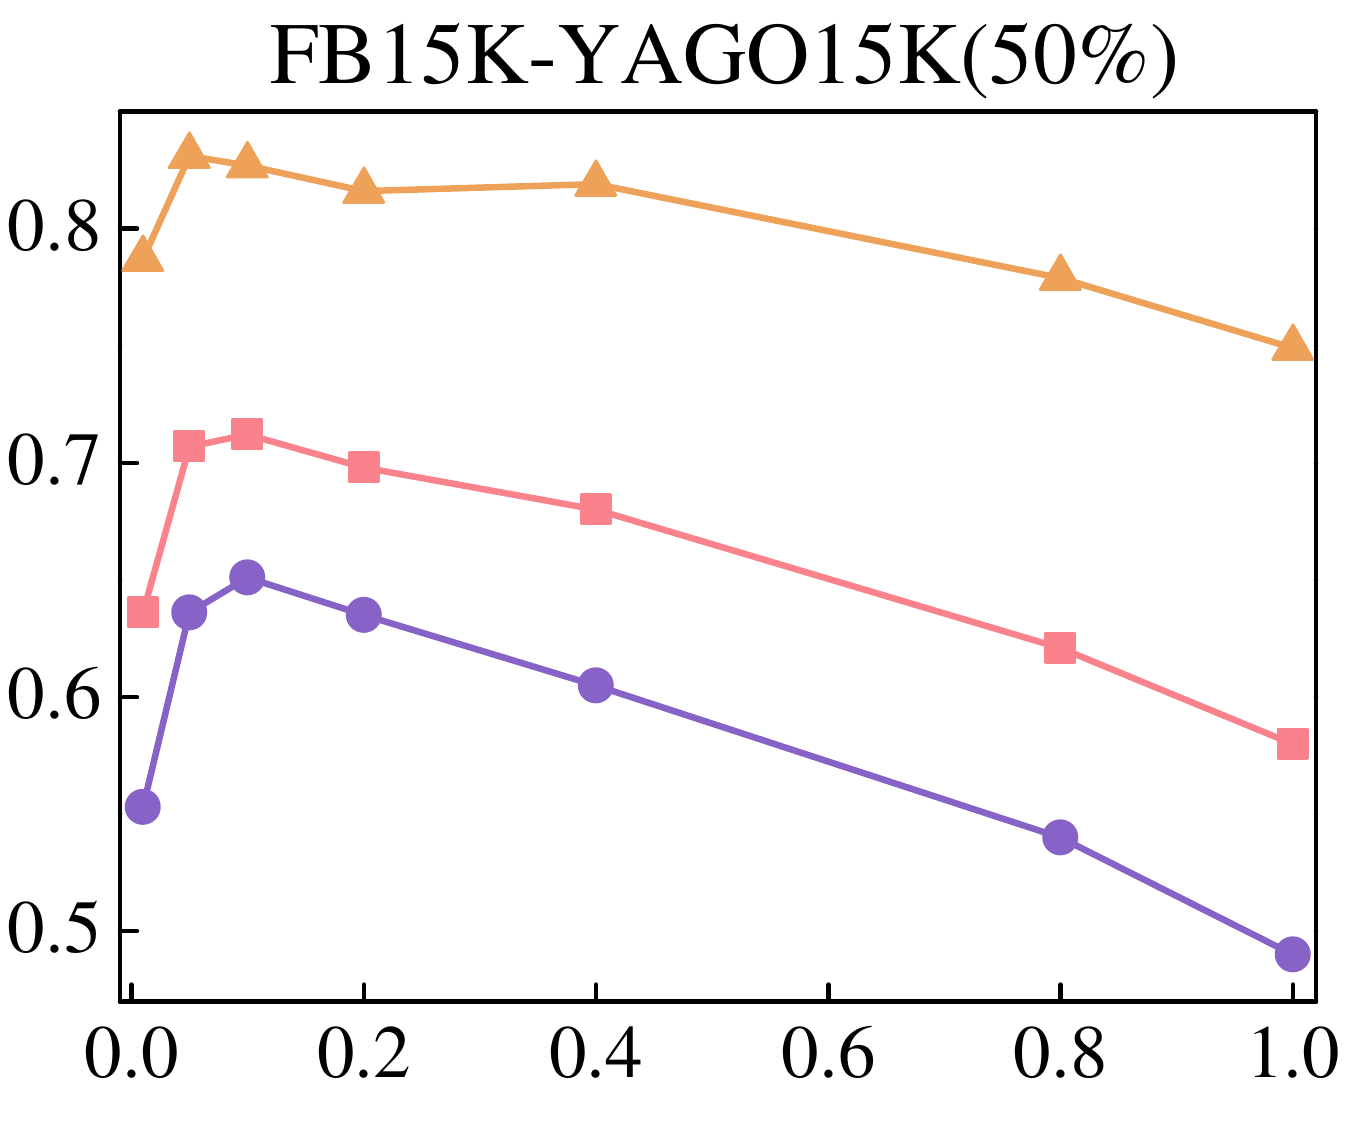}\hfill
  \includegraphics[width=0.16\linewidth]{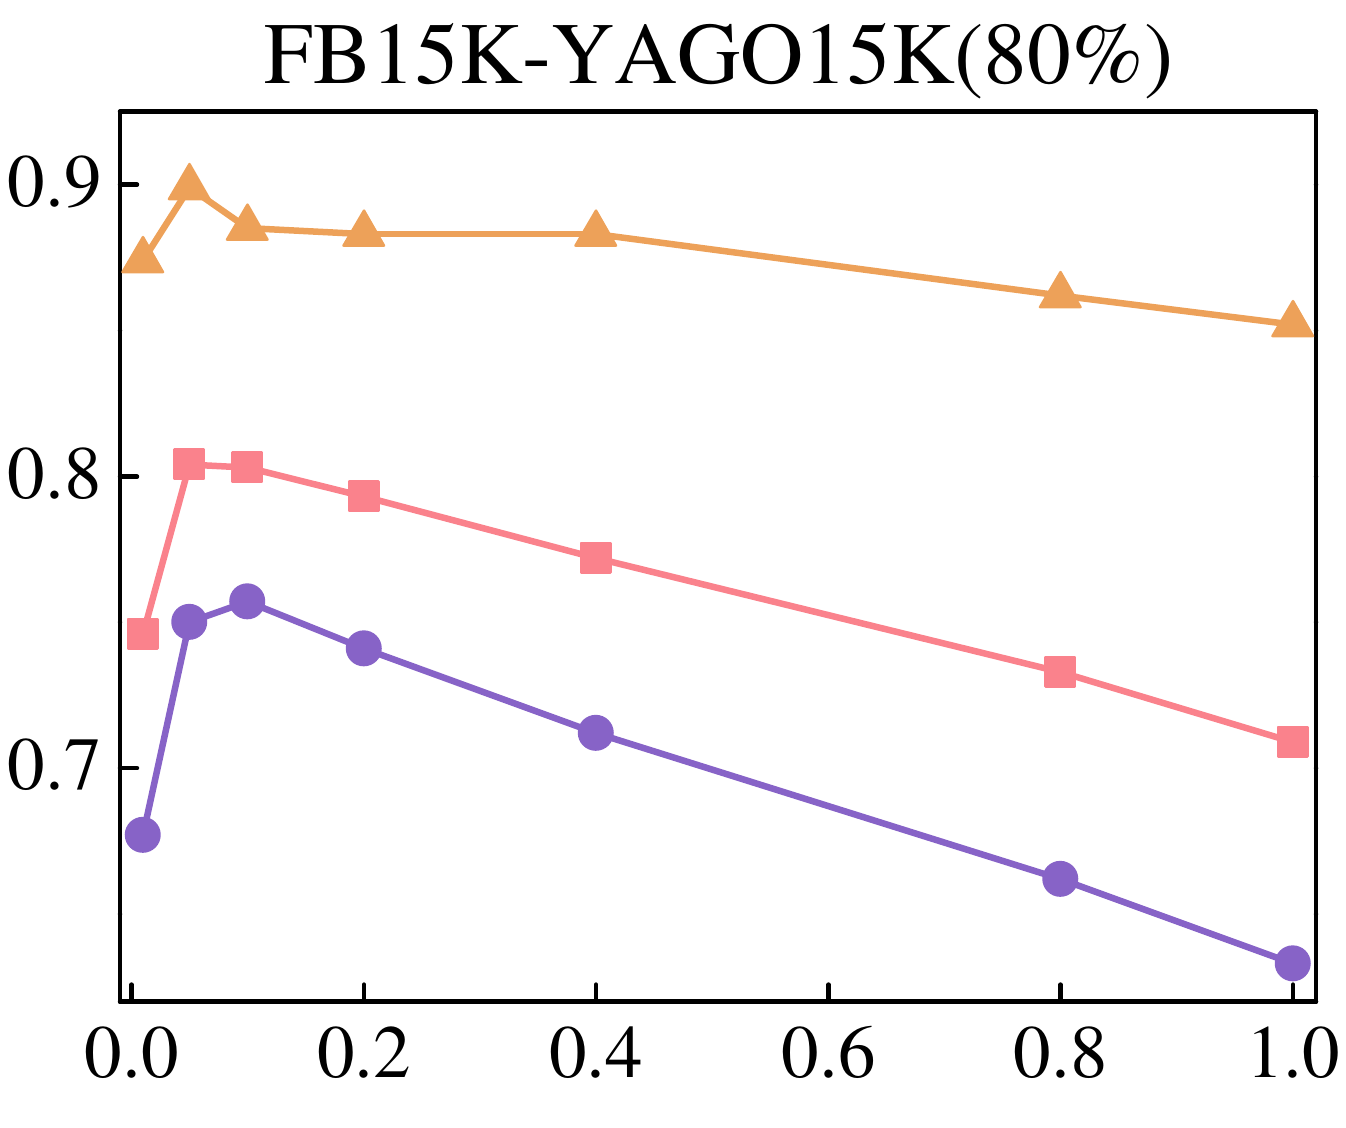}}

  \includegraphics[width=0.25\linewidth]{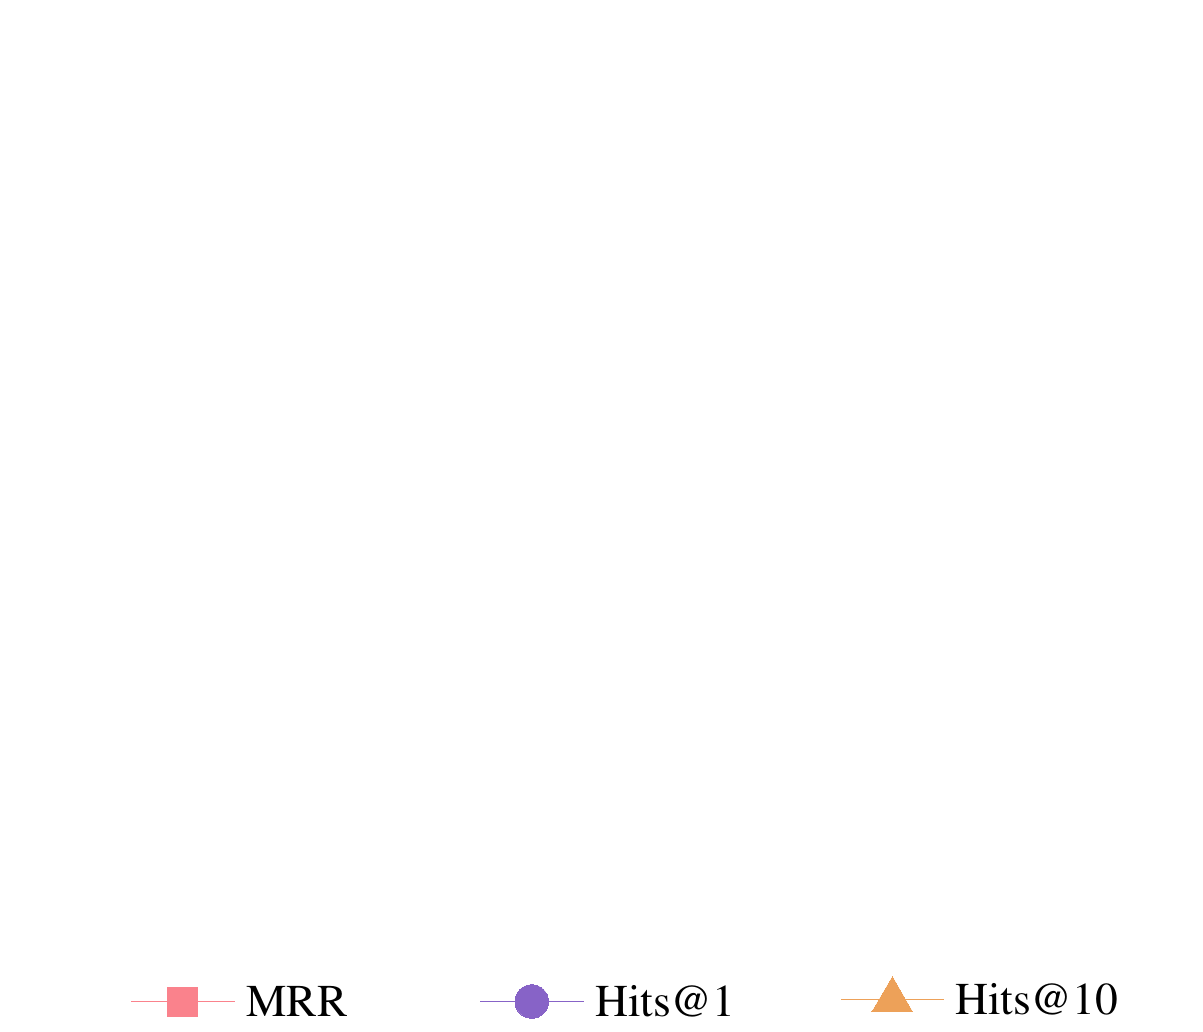}
  \caption{The ablation studies results under different experimental conditions.}
\label{figure_hyper_parameters}
\end{figure*}

\subsection*{A\,\,\,DATASETS}
\hypertarget{datasets}{}
\vic{we conducted experiments on two multi-modal datasets, following previous studies~\citep{Zhenxi_2022, Zhuo_2022, Qian_2023, Lingbing_2023}:  FB15K-DB15K and FB15K-YAGO15K, where FB15K, DB15K, and YAGO15K are extracted from the Freebase~\citep{Kurt_2008}, DBpedia~\citep{Auer_2007}, and YAGO~\citep{Thomas_2016} knowledge bases, respectively. Note that a set of pre-aligned entity pairs are offered for guidance, according to the seed alignment ratio (20\%, 50\%, 80\%). The FB15K-DB15K and FB15K-YAGO15K are proportionally split into training set and testing set. The statistics corresponding to FB15K, DB15K, and YAGO15K are shown in Table~\ref{table_datasets}.}
%For fair comparison, we conduct experiments on two multi-modal datasets following previous studies~\citep{Zhenxi_2022, Zhuo_2022, Qian_2023, Lingbing_2023}, namely FB15K-DB15K and FB15K-YAGO15K, where FB15K, DB15K, and YAGO15K are extracted from the Freebase~\citep{Kurt_2008}, DBpedia~\citep{Auer_2007}, and YAGO~\citep{Thomas_2016} knowledge base, respectively. Note that a set of pre-aligned entity pairs are offered for guidance, according to the seed alignment ratio (20\%, 50\%, 80\%), the FB15K-DB15K and FB15K-YAGO15K are proportionally split into training set and testing set. The statistics corresponding to FB15K, DB15K, and YAGO15K are shown in Table~\ref{table_datasets}.

\begin{table}[!htp]
\setlength{\abovecaptionskip}{0.05cm}

\setlength{\tabcolsep}{0.62em}
\centering
\small
\caption{Statistics for different datasets. \#Ent.: the number of entities, \#Rel.: the number of relations, \#Att.: the number of attribute, \#Rel tri.: the number of relation triples, \#Attr tri.: the number of attribute triples, \#Image: the number of visual images.}
\begin{tabular*}{0.99\linewidth}{@{}ccccccc@{}}
\bottomrule
\textbf{Datasets} &\#Ent. &\#Rel. &\#Att.  &\#Rel tri. &\#Attr tri. &\#Image\\
\hline
\textbf{FB15K} &14,951 &1,345 &116 &592,213 &29,395 &13,444 \\
\textbf{DB15K} &12,842 &279 &225 &89,197 &48,080 &12,837 \\
\textbf{YAGO15K} &15,404 &32 &7 &122,886 &23,532 &11,194 \\
\bottomrule
\end{tabular*}
\label{table_datasets}
\end{table}

\subsection*{B\,\,\,HYPER-PARAMETERS}
\hypertarget{hyper-parameters}{}
\vic{All experiments are carried out on a 32G Tesla V100 GPU, we use the AdamW as the optimizer to update the parameters. We fine-tune the hyper-parameters including the embedding size of modalities $d \in$ \{100, 200, 300, \textbf{400}\}, the learning rate of $lr \in$ \{3e-4, 4e-4, \textbf{5e-4}, 6e-4\}, the incremental rate of the modal weight coefficient $\lambda \in$ \{\textbf{0.1}, 0.2, 0.3, 0.4, 0.5\}, the probability distribution function in PMF module including $\{\textbf{Beta}, Cauchy, Gamma, Gumbel, Laplace\}$, the temperature parameter in contrastive loss $\tau \in$ \{0.01, 0.05, \textbf{0.1}, 0.2, 0.4, 0.8, 1.0 \}, the inner-graph alignment ratio in contrastive loss $\gamma \in$ \{0.6, 0.7, \textbf{0.8}, 0.9, 1.0 \}. The number of training epochs is 1000 with early-stopping and the batch size is 512. Similar to ~\citep{Fangyu_2021, Liyi_2022, Zhenxi_2022, Zhuo_2022}, in the iterative training strategy, in the last 500 epochs of training, every $R=5$ epochs, we select entity pairs that are mutual nearest neighbours in the vector space and add them to the buffer area. After the subsequent $M=50$ epochs, if these entity pairs still exist, we add them to the training set. It should be noted that among the hyper-parameters, the parameters in bold are the configurations selected in our experimental report. We used the same parameter settings on all datasets: FB15K-DB15K and FB15K-YAGO15K datasets.}
%All experiments are carried out on a 32G Tesla V100 GPU, we use the AdamW as the optimizer to update the parameters. We fine-tune the hyper-parameters including the embedding size of modalities $d \in$ \{100, 200, 300, \textbf{400}\}, the learning rate of $lr \in$ \{3e-4, 4e-4, \textbf{5e-4}, 6e-4\}, the incremental rate of the modal weight coefficient $\lambda \in$ \{\textbf{0.1}, 0.2, 0.3, 0.4, 0.5\}, the probability distribution function in PMF module including $\{\textbf{Beta}, Cauchy, Gamma, Gumbel, Laplace\}$, the temperature parameter in contrastive loss $\tau \in$ \{0.01, 0.05, \textbf{0.1}, 0.2, 0.4, 0.8, 1.0 \}, the inner-graph alignment ratio in contrastive loss $\gamma \in$ \{0.6, 0.7, \textbf{0.8}, 0.9, 1.0 \}. The number of training epochs is 1000 with early-stopping and the batch size is 512. Similar to ~\citep{Fangyu_2021, Liyi_2022, Zhenxi_2022, Zhuo_2022}, if under iterative training strategy, in the last 500 epochs of training, every $R=5$ epochs, we select entity pairs that are mutual nearest neighbours in vector space and add them to the buffer area, and after the subsequent $M=50$ epochs, if these entity pairs still exist, we add them to the training set. It should be noted that among the hyper-parameters, the parameters in bold are the configurations selected in our experimental report. We used the same parameter settings on the FB15K-DB15K and FB15K-YAGO15K datasets.

\subsection*{C\,\,\,EVALUATION METRICS}
\hypertarget{evaluation_metrics}{}
\vic{For every entity pair ($e_1$, $e_2$) in the test set, we obtain a ranking list for the possible alignment entities $e_2$. We use three  evaluation metrics: mean reciprocal rank (MRR), and Hits@\textit{k}($k \in \{1, 10\}$). MRR measures the inverse of the rank for the first correct answer, Hits@\textit{k} represents the rate of ecorrect entities ranked in the top-\textit{k} answers. The higher the values of Hits@\textit{k} and MRR, the better performance of the model.}
%For every entity pair ($e_1$, $e_2$) in the test set, we obtain a ranking list for the possible alignment entities $e_2$, and we use three automatic evaluation metrics: mean reciprocal rank (MRR), and Hits@\textit{k}($k \in \{1, 10\}$), MRR measures the inverse of the rank for the first correct answer, Hits@\textit{k} means the rate correct entities rank in the top-\textit{k} answers. The higher values of Hits@\textit{k} and MRR, the better performance of the model.

\subsection*{D\,\,\,PARAMETER ANALYSIS}
\hypertarget{parameter_analysis}{}
\vic{To address \textbf{RQ4}, we investigate the effect of choosing  different hyper-parameters. The results are shown in Figure~\ref{figure_hyper_parameters}.}

\smallskip 
\noindent \textbf{Different  Embedding Dimensions $d$.}
%\subsubsection{Different of Embedding Dimension $d$.} 
\vic{Figure~\ref{figure_hyper_parameters}(a) presents results on the influence of the hidden sizes. We observe that the increase of the hidden sizes helps to capture more messages, which helps to improve the model performance. However, increasing the hidden size will increase the amount of video memory occupied. Thus, in practice, we  might need to find a compromise between performance and computational complexity. }

%Figure~\ref{figure_hyper_parameters}(a) presents results showing the influence of the hidden sizes. We can find that increase of the hidden size helps to capture more messages, which further improve the model performance. However, increasing the hidden size will increase the amount of video memory occupied. We need to make a compromise based on machine performance in practice. 

\smallskip 
 \noindent \textbf{Different  Incremental Rates $\lambda$.}
%\subsubsection{Different of Incremental Rate $\lambda$.} 
%
\vic{The coefficient $\lambda$ in the PMF module is used to scale the calculation results of the KL divergence. Figure~\ref{figure_hyper_parameters}(b) shows that the value of  $\lambda$ does not have a decisive impact on the performance, showing that  MMIEA's robustness in this respect. }
%We introduce the coefficient $\lambda$ in the PMF module to appropriately scale the calculation results of KL divergence. As shown in Figure~\ref{figure_hyper_parameters}(b), $\lambda$ does not have a decisive impact on the overall performance of MMIEA. This indicates that MMIEA exhibits a certain level of robustness with respect to the numerical values of KL divergence calculations. 

\smallskip 
 \noindent \textbf{Different  Weight Values $\gamma$.}
%\subsubsection{Different of Weight Value $\gamma$.} 
\vic{The weight coefficient $\gamma$ in Equation~\eqref{equation_9} is used to adjust the importance level of positive and negative samples between the inner-graph and cross-graph for a modality.  Figure~\ref{figure_hyper_parameters}(c) shows the results for different weight values. We can observe that variation of the weight coefficient  only brings  subtle performance differences.}
%The weight coefficient $\gamma$ in Equation~\ref{equation_9} can be used to adjust the importance level of positive and negative samples between the inner-graph and cross-graph within the modality. The corresponding results for different weight values are shown in Figure~\ref{figure_hyper_parameters}(c). We can find that the selection of the contrastive learning weight coefficient will only bring about subtle performance differences, so the MMIEA has strong adaptability to the selection of the $\gamma$.

\smallskip 
 \noindent \textbf{Different Temperature Values $\tau$.}
%\subsubsection{Different of Temperature Value $\tau$.} 
\vic{The temperature coefficient adjusts the similarity distribution between contrastive embeddings. It affects the performance of contrastive learning models by expanding or shrinking the relative distance between different samples in the embedding space. Figure~\ref{figure_hyper_parameters}(d) shows  that setting different temperature coefficients has significant impact on MMIEA. A higher temperature coefficient makes the difference between similarity scores smoother, making the samples harder to distinguish.  Although lower temperatures might make it easier for the model to distinguish different samples, it will increase the model's sensitivity. So, in practice, we need to choose a temperature coefficient that ensures a  balance between the stability and flexibility of the model.}

%The temperature coefficient can be used to adjust the similarity distribution between contrastive embeddings. It affects the performance of contrastive learning models by expanding or shrinking the relative distance between different samples in the embedding space. From Figure~\ref{figure_hyper_parameters}(d), it can be observed that seeing different temperature coefficients has significant impact on MMIEA. A higher temperature coefficient tends to cause the differences between similarity scores to be smoother, making the samples more harder to distinguish. Conversely, when the temperature coefficient is lower, the differences between similarity scores is more obvious. Although it can make it easier for the model to distinguish different samples, it will increase the model's sensitivity. In practice, we need to strike a balance between the stability and flexibility of the model to choose an appropriate temperature coefficient.
